# Supplementary material for: Efficient Memory Partitioning in Software Defined Hardware
Source: arXiv:2202.01261 source file (2022-03-29)
Supplement: Supplementary file 1 [file appendices.pdf]

# Appendices

Anonymous Author(s)

## A Model Learning Curves and Parameters

Figures 1, 2, and 3, as well as Table 1 show the learning curves and parameters for the ML model.

## B Bank Offset Correction Calculation

As far as we are aware, prior papers outlining the implementation of the bank resolution equations (Equations 1 and 2) do not explicitly provide a formula for addressing intra-bank offset when when B > 1. When B = 1, the neighborhood vector, $\vec{P}$ scopes out a hypercube where each bank is represented once. When B > 1 then $\vec{P}$ must be selected such that each bank appears *at most* B times.

The intuition behind the intra-bank correction, $C$, in Equation 2 comes from the idea of periodicity per-dimension in the bank address equation (Equation 1) Equation 1 shows how to use the least-common multiple of certain parameters to compute this periodicity, $\vec{\Phi}$.

$$\vec{\Phi}_i = \frac{lcm(\vec{\alpha}_i, NB)}{\vec{\alpha}_i} \tag{1}$$

Because intra-bank offset (Equation 2) depends on floor division of an address by $B$ under modulo $N$, we are guaranteed that no neighborhood can contain more than $B$ unique instances of a single bank because of this periodicity. Computing the dot product $\vec{x} \cdot \vec{\alpha}$ and applying modulo $B$ to this quantity distinguishes multiple instances of the same bank in a neighborhood uniquely. In cases where $\alpha_i$ and $NB$ are not co-prime (i.e. $\Phi_i < NB$), then it is possible to substitute $B$ with $\lceil \frac{\vec{\Phi}_i}{B} \rceil$ in the intra-bank offset calculations.

Consider the simple example in Figure 4 for N = 4, B = 2, $\alpha$ = 3, and P = $\Phi$ = 8. The color of each cell represents its bank and the intra-bank offset is labeled with an integer over the cell. The intra-bank correction is required so that no cells of the same bank have the same intra-bank offset.

*PLDI'20, June 15–20, 2020, London, United Kingdom*
2020.

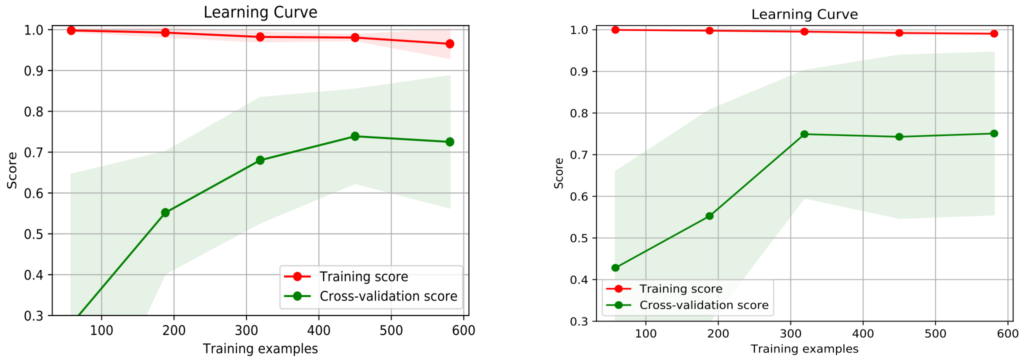


**(a)** The baseline model. **(b)** The proposed pipeline.

**Figure 1.** Learning curves of the baseline model (left) and our proposed model pipeline when predicting FF utilization.

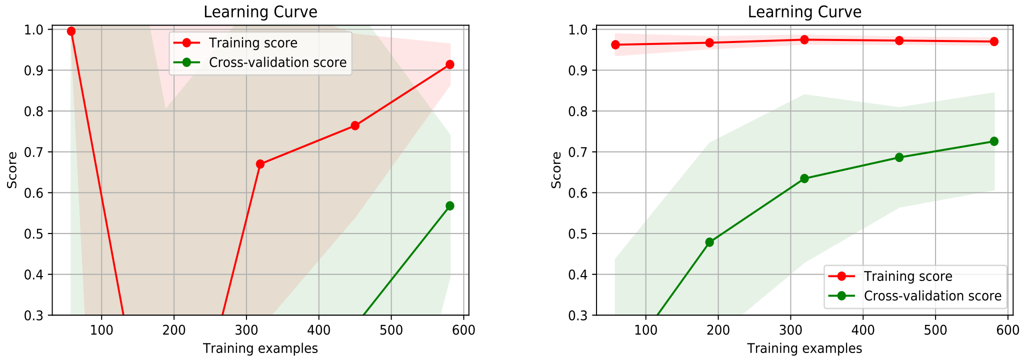


**(a)** The baseline model. **(b)** The proposed pipeline.

**Figure 2.** Learning curves of the baseline model (left) and our proposed model pipeline when predicting RAMB18 utilization. The baseline model starts to overfit on the dataset despite of all the regularization introduced. However, our pipeline still manages to achieve high performance without overfitting.

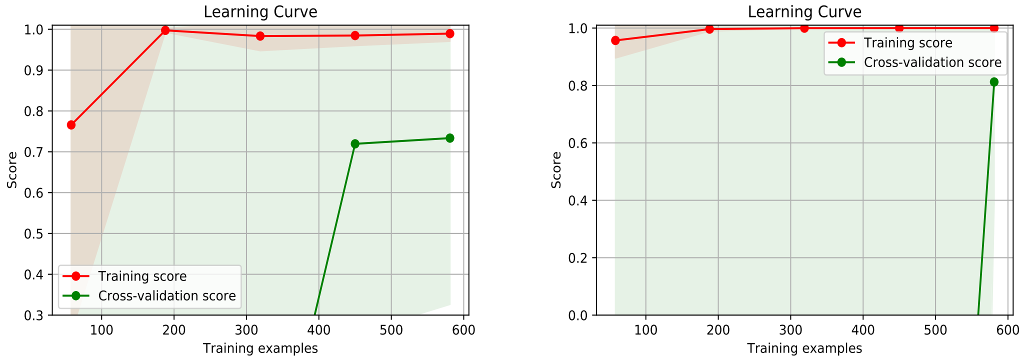


**(a)** The baseline model. **(b)** The proposed pipeline.

**Figure 3.** Learning curves of the baseline model (left) and our proposed model pipeline when predicting RAMB36 utilization. We observed that the FPGA PnR tool mapped small memory to RAMB36 less frequently. Hence, the training data for RAMB36 is much less than the other resource types. As a result, the standard deviations for both models are very high.

| Model | Model architecture | | Training parameters | | Regularization parameters | |
|---|---|---|---|---|---|---|
| Ours | **random state** | 30 | **objective** | mean-squared error | **subsample** | 0.6 |
| | **number of estimators** | 159 | **learning rate (lr)** | 0.1 | **col sample by tree** | 1 |
| | **max tree depth** | 3 | | | $\lambda$ | 0.04 |
| | **min samples split** | 10 | | | $\alpha$ | 3 |
| | | | | | $\gamma$ | 5 |
| MLP | **hidden states** | [128, 32, 32, 16] | **objective** | mean-squared error | $\alpha$ | 0.07 |
| | **activation** | *relu* | **learning rate (lr)** | adaptive | | |
| | | | **initial lr** | 0.0015 | | |
| | | | **power_t** | 0.5 | | |

**Table 1.** Final parameters of the evaluated models.

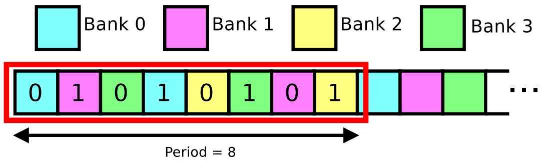


**Figure 4.** Example showing how intra-bank offset correction properly labels an example where N=4, B = 2, $\alpha$ = 3 and P = $\Phi$ = lcm(3,4*2)/3 = 8.
